# Supplementary material for: Relativistic response and novel spin-charge plasmon at the Tl/Si(111) surface
Source: arXiv:1704.07273 ancillary file (2017-04-24)
Supplement: Supplementary file 1 [file supplemental_material.pdf]

# Supplemental material for “Relativistic response and novel spin-charge plasmon at the Tl/Si(111) surface”

Jon Lafuente-Bartolome,<sup>1,2</sup> Idoia G. Gurtubay,<sup>1,2</sup> and Asier Eiguren<sup>1,2</sup>

<sup>1</sup>*Materia Kondentsatuaren Fisika Saila, Euskal Herriko Unibertsitatea UPV/EHU, 644 Postakutza, 48080 Bilbao, Basque Country, Spain*

<sup>2</sup>*Donostia International Physics Center (DIPC), Paseo Manuel de Lardizabal 4, 20018 Donostia-San Sebastian, Basque Country, Spain*

(Dated: February 21, 2017)

## S1. WANNIER INTERPOLATION OF THE DENSITY-DENSITY RESPONSE FUNCTION

In this section we briefly account for the description of the Wannier-interpolation technique employed throughout this work in order to efficiently compute the dispersion of the density-density response function with high momentum and energy resolution.

The starting point of the procedure is a self-consistently obtained set of energies ( $\epsilon_{n\mathbf{k}}$ ) and Bloch wave functions ( $|\Psi_{n\mathbf{k}}\rangle$ ) over a relatively coarse Monkhorst-Pack  $\mathbf{k}$ -mesh on the first Brillouin zone. Consider now a set of maximally localized Wannier functions, obtained by the procedure described in [1–3],

$$W_{n\mathbf{R}}(\mathbf{r}) = \frac{1}{N_k} \sum_{\mathbf{k}} e^{-i\mathbf{k}\mathbf{R}} \tilde{\Psi}_{n\mathbf{k}}(\mathbf{r}) = \frac{1}{N_k} \sum_{\mathbf{k}} e^{-i\mathbf{k}\mathbf{R}} \sum_m^M U_{mn}^{\mathbf{k}} \Psi_{m\mathbf{k}}(\mathbf{r}) , \quad (1)$$

where  $N_k$  represents the number of  $\mathbf{k}$ -points on the initial mesh, the  $U_{mn}^{\mathbf{k}}$ -s are the unitary matrices which fix the gauge of the Bloch functions so that  $W_{n\mathbf{R}}(\mathbf{r})$  are maximally localized in real space, and  $\tilde{\Psi}_{\mathbf{k},n}(\mathbf{r})$  are the Wannier-Bloch wave functions, which are maximally flat in reciprocal space by construction. For simplicity we have considered here an isolated manifold of  $M$  bands.

We can now construct the matrix elements entering the expression of  $\chi^0$  (see Eq.(3) of main text) in the basis of the Wannier-Bloch wave functions (omitting the spin indexes here for simplicity),

$$Z_{mn}^{\mathbf{k}(W)}(\mathbf{q}, \mathbf{G}) = \langle \tilde{\Psi}_{m\mathbf{k}} | e^{i(\mathbf{q}+\mathbf{G})\mathbf{r}} | \tilde{\Psi}_{n\mathbf{k}+\mathbf{q}} \rangle = \sum_{ij} (U^{\mathbf{k}})_{mi}^{\dagger} \langle \Psi_{i\mathbf{k}} | e^{i(\mathbf{q}+\mathbf{G})\mathbf{r}} | \Psi_{j\mathbf{k}+\mathbf{q}} \rangle U_{jn}^{\mathbf{k}+\mathbf{q}} , \quad (2)$$

which after computing them in the coarse  $\mathbf{k}$ -mesh, can be effectively evaluated at an arbitrary  $\mathbf{k}'$  point outside the initial mesh exploiting their flatness in  $\mathbf{k}$  space by means of a Fourier interpolation,

$$Z_{mn}^{\mathbf{k}'(W)}(\mathbf{q}, \mathbf{G}) = \sum_{\mathbf{R}} \sum_{\mathbf{k}} e^{i(\mathbf{k}'-\mathbf{k})\mathbf{R}} Z_{mn}^{\mathbf{k}(W)} . \quad (3)$$

We can then rotate the matrix elements back to the Bloch gauge by using the unitary matrices obtained in the diagonalization of the Wannier-Bloch Hamiltonian (which is constructed in a similar way) at the  $\mathbf{k}'$  point,

$$\sum_{ij} (\tilde{U}^{\mathbf{k}'} )_{mi}^\dagger H_{ij}^{\mathbf{k}'(W)} \tilde{U}_{jn}^{\mathbf{k}'} = \delta_{mn} \epsilon_{n\mathbf{k}'} . \quad (4)$$

From Eq.(4) we also obtain the interpolated energies (and therefore the occupation factors  $f_{n\mathbf{k}'}$ ), which enter the expression of  $\chi^0$ . By following this procedure, we are able to obtain a very dense sampling of all the  $\mathbf{k}$ -dependent quantities entering the summation of Eq.(3) in the main text, allowing for a well-converged calculation of  $\chi^0$  at an affordable computational cost.

Finally, in order to obtain a smooth momentum dispersion of the response matrix, we can directly interpolate the Wannier-Bloch wave function in its real-space representation to an arbitrary  $\mathbf{k}' = \mathbf{k} + \mathbf{q}'$  point,

$$\tilde{\Psi}_{n\mathbf{k}'}(\mathbf{r}) = \sum_{\mathbf{R}} \sum_{\mathbf{k}''} e^{i(\mathbf{k}' - \mathbf{k}'')\mathbf{R}} \tilde{\Psi}_{n\mathbf{k}''}(\mathbf{r}) , \quad (5)$$

and after computing the matrix elements  $Z_{mn}^{\mathbf{k}(W)}(\mathbf{q}', \mathbf{G}) = \langle \tilde{\Psi}_{m\mathbf{k}} | e^{i(\mathbf{q}' + \mathbf{G})\mathbf{r}} | \tilde{\Psi}_{n\mathbf{k} + \mathbf{q}'} \rangle$ , follow the very same procedure for the interpolation in  $\mathbf{k}$ .

## S2. GENERALIZED SPIN-CHARGE DENSITY-DENSITY RESPONSE MATRIX

In this section we show the macroscopic contributions of all the 16 elements of the generalized spin-charge density response matrix at the hole-doped ( $-30$  meV) Tl/Si(111) surface, as obtained by means of our all-electron relativistic calculations. We show in Fig.1 (Fig.2) the imaginary parts of the non-interacting (full-interacting) response tensor elements, which relate the induced charge and spin densities and the effective (external) electromagnetic field (see Eq.(6) of the main text).

We see in Fig.1 that in the case of the Tl/Si(111) surface, the spin-charge response tensor roughly follows the behavior of a pure Rashba-like system [4]. Nevertheless, due to the anisotropy of the Fermi surface and the non-zero perpendicular component of the spin-polarization of the surface states, we can appreciate a non-zero (though considerably smaller) intensity in the  $\chi_{\text{KS}}^{y0}$ ,  $\chi_{\text{KS}}^{0y}$ ,  $\chi_{\text{KS}}^{z0}$ ,  $\chi_{\text{KS}}^{0z}$ ,  $\chi_{\text{KS}}^{xy}$ ,  $\chi_{\text{KS}}^{yx}$ ,  $\chi_{\text{KS}}^{xz}$  and  $\chi_{\text{KS}}^{zx}$  responses, and their full-interacting counterparts (see Fig.2). Even if the  $\omega_q \sim \sqrt{q}$  dispersing peak is recognizable in  $\text{Im}(\chi^{0y})$ ,  $\text{Im}(\chi^{xy})$ ,  $\text{Im}(\chi^{yx})$  and  $\text{Im}(\chi^{yy})$ , its intensity is considerably smaller in magnitude and its contribution to the spin character of the collective oscillation is negligible, as we shall see in the next section.

### S3. REAL-SPACE REPRESENTATION OF THE FOUR-COMPONENT SELF-SUSTAINED COLLECTIVE OSCILLATION

As already mentioned in the main text, in order to resolve in detail the spatial configuration and the mixed spin-charge character of the collective excitation, we rewrite the equation of the dielectric response matrix,

$$\delta\phi^{\mu,\mathbf{G}(\text{ext})} = \sum_{\nu} \sum_{\mathbf{G}'} \epsilon^{\mu\nu,\mathbf{G}\mathbf{G}'} \delta\phi^{\nu,\mathbf{G}'(\text{sc})} , \quad (6)$$

as an eigenvalue equation,

$$\sum_{\nu} \sum_{\mathbf{G}'} \epsilon^{\mu\nu,\mathbf{G}\mathbf{G}'}(\mathbf{q}, \omega) \delta\phi_i^{\nu,\mathbf{G}'}(\mathbf{q}, \omega) = \epsilon_i(\mathbf{q}, \omega) \delta\phi_i^{\mu,\mathbf{G}}(\mathbf{q}, \omega) . \quad (7)$$

The self-sustained collective oscillations ( $\delta\phi^{(\text{ext})} = 0$ ) thus correspond to solutions of Eq.(7) with a vanishing eigenvalue ( $\epsilon_i(\mathbf{q}, \omega) = 0$ ) at each momentum-transfer vector  $\mathbf{q}$  and energy  $\omega$ . The eigenvector corresponding to such a solution will be composed by four elements for each reciprocal lattice vector  $\mathbf{G}$ ,

$$\delta\phi_i^{\mu,\mathbf{G}} = \begin{pmatrix} \delta V_0^{\mathbf{G}} \\ \delta B_x^{\mathbf{G}} \\ \delta B_y^{\mathbf{G}} \\ \delta B_z^{\mathbf{G}} \end{pmatrix}_i , \quad (8)$$

and the real-space representation of the oscillation can be then obtained by a Fourier transformation,

$$\delta\phi_i^{\mu}(\mathbf{r}) = \sum_{\mathbf{G}} e^{-i(\mathbf{q}+\mathbf{G})\cdot\mathbf{r}} \delta\phi_i^{\mu,\mathbf{G}} . \quad (9)$$

We show in Fig.3 the  $z$  and  $\mathbf{q}$  dependence of the four-component self-sustained collective oscillation, represented in the same scale for better comparison. As described in the main text, we can appreciate a strong oscillation of both the charge ( $\delta V_0$ ) and the transverse-spin ( $\delta B_x$ ) components of the induced electromagnetic field, localized in the first few atomic layers close to the surface. A finite longitudinal-spin component ( $\delta B_y$ ) of the oscillation is also appreciable in Fig.3(c), though much smaller in magnitude. We represent in Fig.4 a zoom of the longitudinal-spin component ( $\delta B_y$ ) in its corresponding scale, where we note that the magnitude of this component of the oscillation is  $\sim 20$  times smaller than the transverse-spin component. The perpendicular-spin component ( $\delta B_z$ ) of the oscillation is negligible over the considered momentum range.

- 
- [1] N. Marzari and D. Vanderbilt, Phys. Rev. B **56**, 12847 (1997).
  - [2] I. Souza, N. Marzari, and D. Vanderbilt, Phys. Rev. B **65**, 035109 (2001).
  - [3] A. A. Mostofi, J. R. Yates, G. Pizzi, Y.-S. Lee, I. Souza, D. Vanderbilt, and N. Marzari, Computer Physics Communications **185**, 2309 (2014).
  - [4] S. Maiti, V. Zyuzin, and D. L. Maslov, Phys. Rev. B **91**, 035106 (2015).

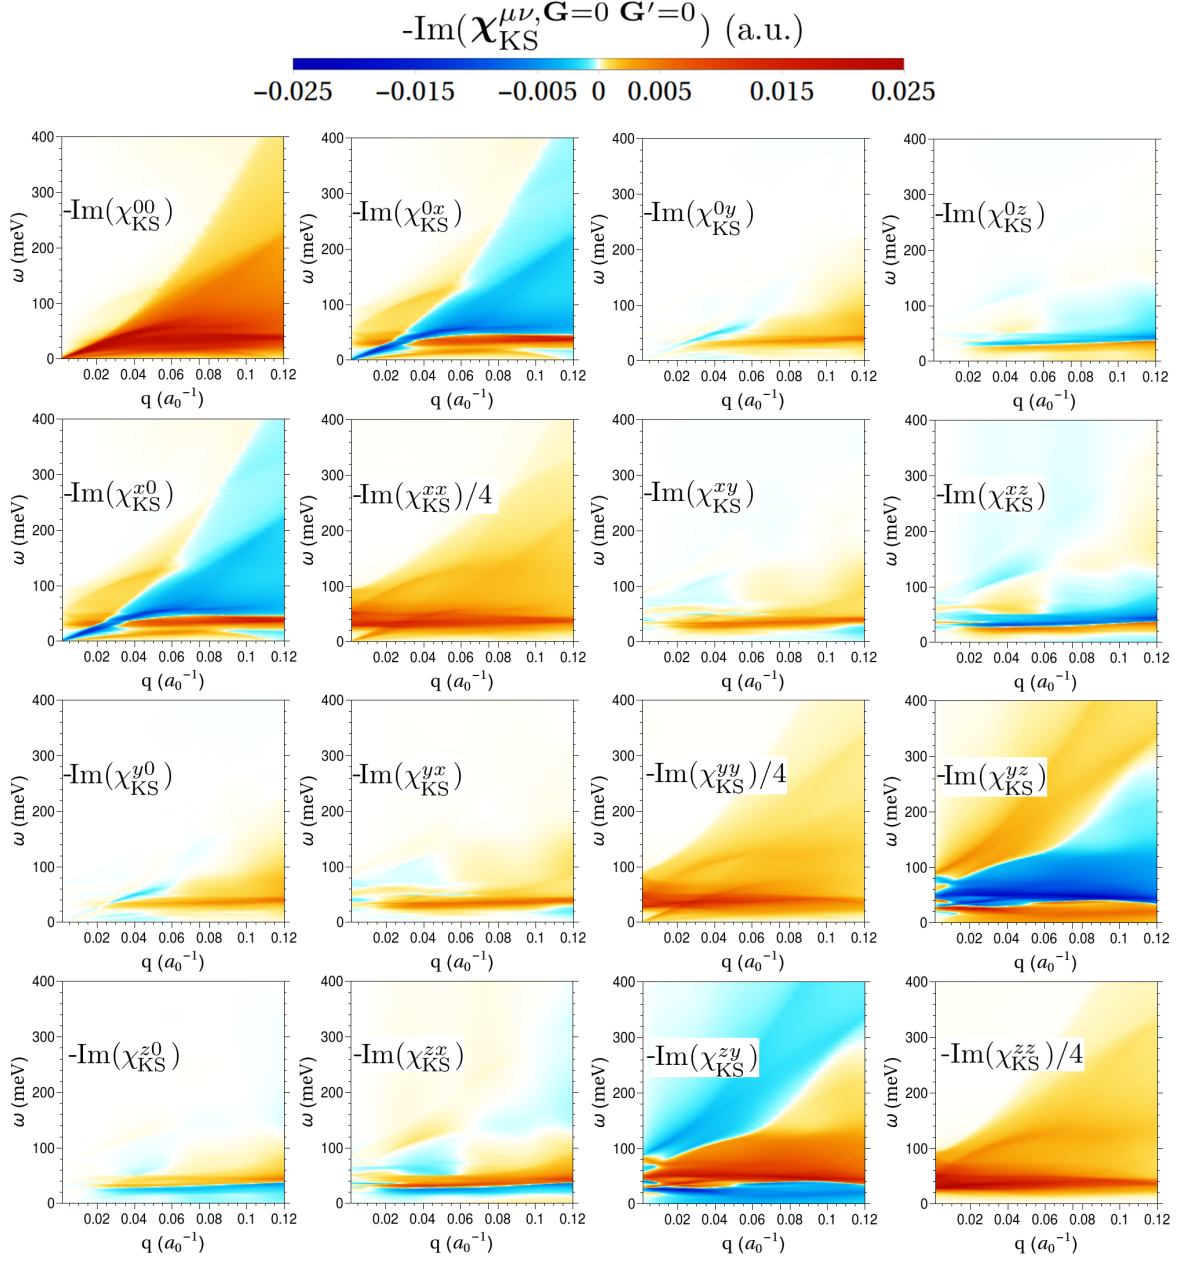

FIG. 1: First-principles calculation of the non-interacting generalized spin-charge density response matrix at the hole-doped Tl/Si(111) surface in the  $\omega \in [0, 400]$  meV energy and  $|\mathbf{q}| \in [0, 0.12]$   $a_0^{-1}$  momentum range, with  $\mathbf{q}$  along the  $\bar{\Gamma} - \bar{M}$  direction (cartesian  $y$  axis in our coordinate system). The color code represents the imaginary part of the macroscopic contribution ( $\chi_{\text{KS}}^{\mu\nu, \mathbf{G}=0 \mathbf{G}'=0}(\mathbf{q}, \omega)$ ) of the response in atomic units, within the scale given by the color bar.

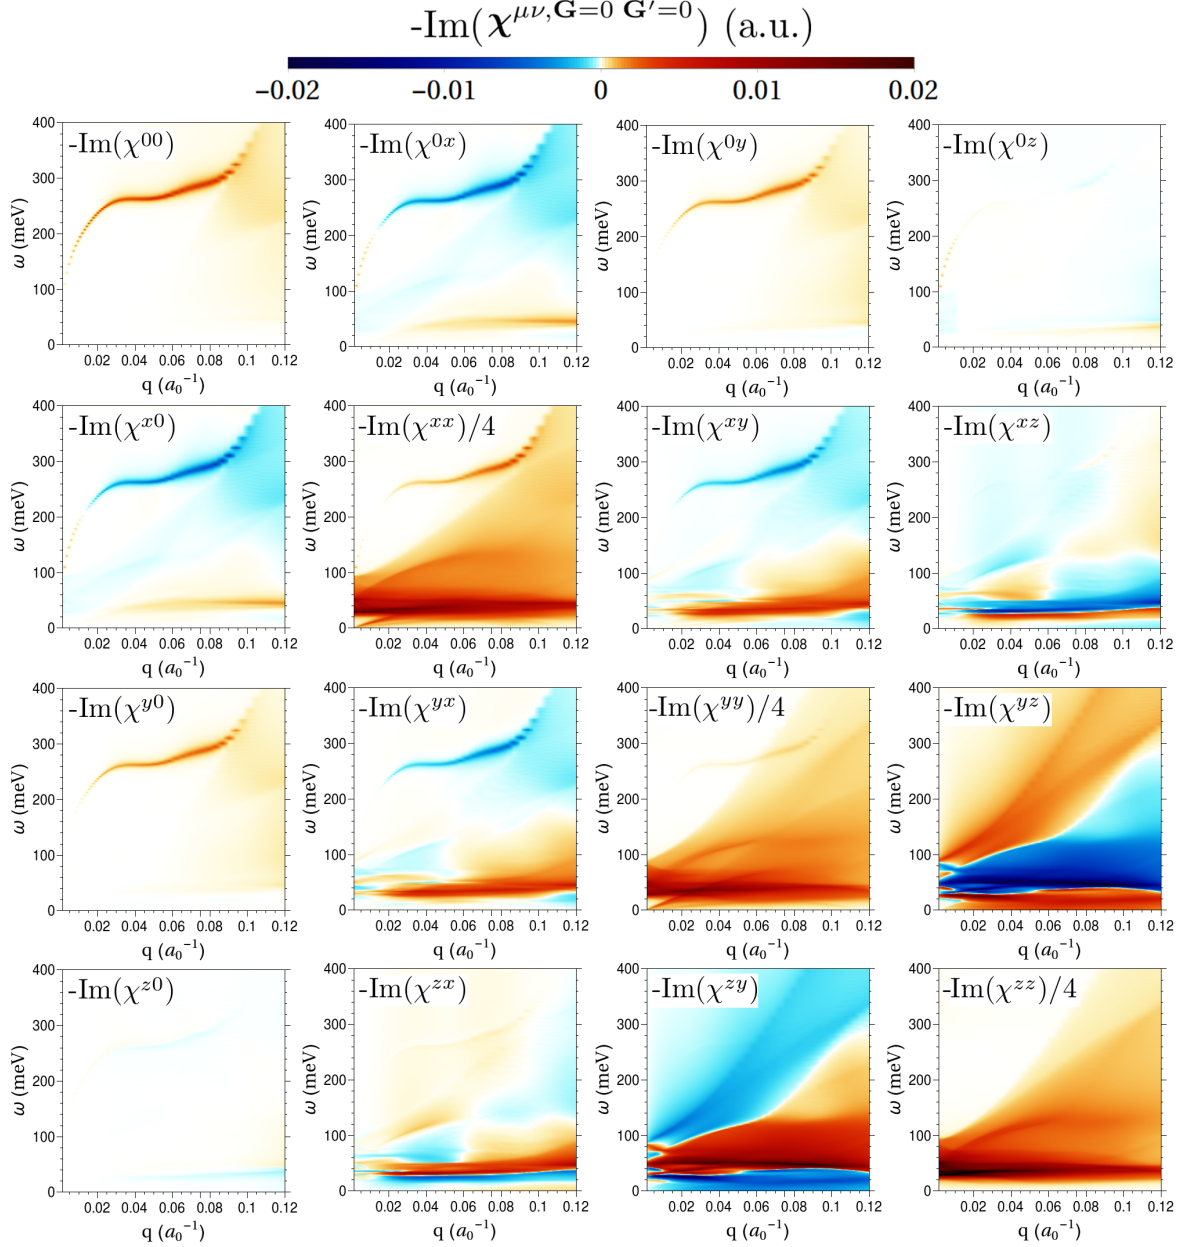

FIG. 2: First-principles calculation of the full interacting generalized spin-charge density response matrix at the hole-doped Tl/Si(111) surface in the  $\omega \in [0, 400]$  meV energy and  $|\mathbf{q}| \in [0, 0.12]$   $a_0^{-1}$  momentum range, with  $\mathbf{q}$  along the  $\bar{\Gamma} - \bar{M}$  direction (cartesian  $y$  axis in our coordinate system). The color code represents the imaginary part of the macroscopic contribution ( $\chi^{\mu\nu, G=0 G'=0}(\mathbf{q}, \omega)$ ) of the response in atomic units, within the scale given by the color bar.

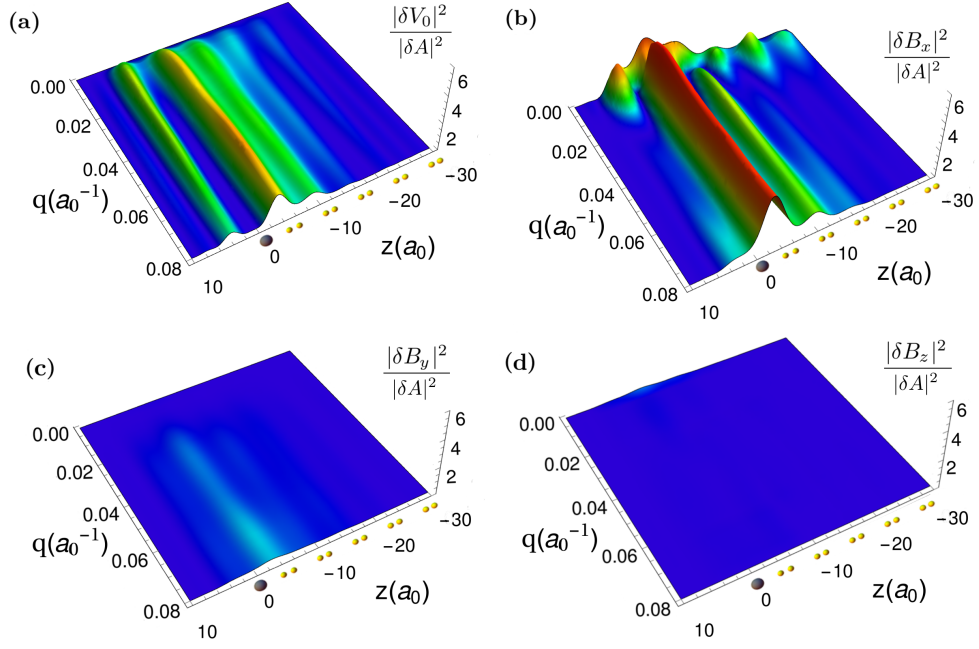

FIG. 3: Real space configuration and  $|\mathbf{q}|$  dependence of the hybrid spin-charge collective oscillation at the Tl/Si(111) surface in the  $\mathbf{q} \in [0, 0.08] a_0^{-1}$  momentum range. (a),(b),(c),(d) Magnitudes of the induced charge potential, transverse magnetic field, longitudinal magnetic field, and perpendicular magnetic field oscillations, respectively, with  $|\delta A|^2 = \int_{cell} d^3r \sum_{\mu} (\delta\phi(\mathbf{r})^{\mu})^* \delta\phi(\mathbf{r})^{\mu}$ . The  $z$  coordinate corresponds to the direction perpendicular to the surface, with negative values indicating penetration into the bulk. Orientative positions of the first thallium and silicon atomic layers are represented by big gray and small yellow spheres, respectively.

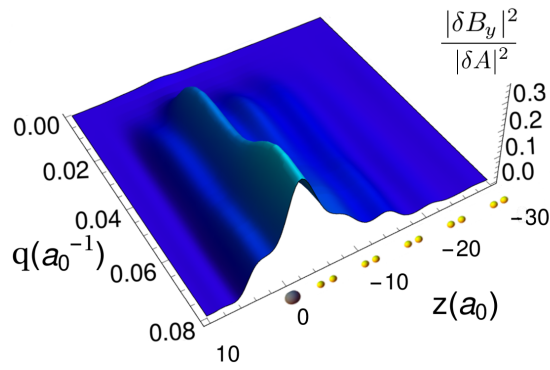

FIG. 4: Zoom of the induced longitudinal magnetic field oscillation, with  $|\delta A|^2 = \int_{cell} d^3r \sum_{\mu} (\delta\phi(\mathbf{r})^{\mu})^* \delta\phi(\mathbf{r})^{\mu}$ .
